# Supplementary material for: Multi-Objective Optimization of Consumer Group Autoscaling in Message Broker Systems
Source: arXiv:2402.06085 source file (2024-02-08)
Supplement: Supplementary file 1 [file modified_any_fit.tex]

\section{Modified Any Fit Algorithm}
